# Supplementary material for: Hybrid Gromov-Wasserstein Embedding for Capsule Learning
Source: arXiv:2209.00232 source file (2023-10-24)
Supplement: Supplementary file 1 [file Supplementary.pdf]

## Appendix

### ( A.1.)

**Proposition 1.** *In the special case when the learning rate is  $1/\eta$ , the problem (5) can be solved by regularized optimal transport.*

*Proof.* As shown by [1], the regularized optimal transport problem can be presented as

$$\min_{T \in \Gamma(\Omega_p, \Omega_q)} \langle C^{(\mathcal{U}, \mathcal{V})}, T \rangle - \eta H(T), \quad (4a)$$

where,  $C^{(\mathcal{U}, \mathcal{V})} = L(C_p, C_q, T^{(\mathcal{V})}) + \beta K(X_p^{\mathcal{U}}, X_q^{\mathcal{U}}) + \eta$ , and  $H(T) = -\sum_{ij} \log(T_{ij})$ . This regularization yields favorable computational properties since defines a convex algorithm that involves a Sinkhorn projection [2], by only performing matrix-vector multiplications. In this case, each updating step (4) can be solved via projected gradient descent, which is a solution to a regularized optimal transport problem (4a).

### ( A.2. )

Beyond the significant performance improvement, one of the advantages of the proposed capsule model is its computational efficiency. Learning optimal transport is computationally hard in the general case, due to the tensor-matrix multiplication  $L(C_p, C_q, T)$ . To provide a successful learning process, Peyré et al. [3] suggested an efficient way to compute  $L(.,.)$  as

$$L(a, b) = f_1(a) + f_2(b) - h_1(a)h_2(a) \quad (1)$$

for functions  $(f_1, f_2, h_1, h_2)$ , then for any  $T \in \Gamma(\Omega_p, \Omega_q)$ , the computation problem can be rewritten as

$$L(C_p, C_q, T) = \Gamma_{C_p, C_q} - h_1(C_p)Th_2(C_q)^T. \quad (2)$$

where  $\Gamma_{C_p, C_q} = f_1(C_p)\Omega_p 1_{V_q}^T + f_2(C_q)^T 1_{V_p}\Omega_q^T$ , which is independent of  $T$ . Formula (2) shows that for this class of losses, we can compute  $L(.)$  efficiently in  $\mathcal{O}(M^2D + M^3N)$ , for  $M = \{V_p, V_q\}$ , which can be simplified as: the complexity of distance matrix would be  $M^2D$ , and for the optimal transport is  $NM^3$ . This process only requires matrix multiplication and is best suited for for parallel computing on GPUs.

## ( A.3.)

For the layer  $k$ , suppose  $x$  is an input feature vector from lower layer  $k-1$ , with the ground truth label  $y \in \{1, 2, \dots, L\}$ . Given a set of capsule vectors  $\{v_1, v_2, \dots, v_L\}$  corresponding to a feature vector  $x$  and group of SubCapsules  $v_y$ , we train the model as,  $\|v_y\|_2 > \|v_l\|_2$ . That means, we require  $\|v_y\|$  should be larger than all the length of the other capsules (i.e.,  $\|v_y\|$  are those capsules  $a$  that are highly aligned with the input). We provide a general framework for the summation-based family of routing procedures in Algorithm 1.

---

**Algorithm 1** Training of the proposed WECapsule. Our algorithm returns the activation and poses of the capsules in layer  $k+1$  based on the alignment score in layer  $k$ ; the capsules are activated for the upper layers by finding the alignment between the input and SubCapsule sets.

---

**Input:**  $\{C_p, \Omega_p\}, \{C_q, \Omega_q\}, \lambda, \eta$ , number of outer-inner iterations  $\{\mathcal{U}, \mathcal{V}\}$ .

**Output:**  $X_p, X_q$  and  $\bar{T}$ .

**For**  $\mathcal{U} = 0$  to  $U-1$

    Set  $\bar{\beta}_{\mathcal{U}} = \frac{\mathcal{U}}{U}$ .

**For**  $\mathcal{V} = 0$  to  $N-1$

        Update optimal transport  $\bar{T}^{(\mathcal{U}+1)}$  via Eq.(5).

        Obtain  $X_p^{(\mathcal{U}+1)}, X_q^{(\mathcal{U}+1)}$  via Eq.(6).

$X_p = X_p^{(\mathcal{U})}, X_q = X_q^{(\mathcal{U})}, \bar{T} = \bar{T}^{(\mathcal{U})}$ .

$\backslash\backslash$  we set the correspondence/alignment  $\mathcal{A} = \emptyset$

**For**  $v_i \in V_p$

$j = \argmax_j \bar{T}_{ij}$ .  $\mathcal{A} = \mathcal{A} \cup \{(v_i \in V_p, v_j \in V_q)\}$ .

---

## B.1. Classification Accuracy on CIFAR10 and FashionMNIST

We compare our classification model, with four CapsNet-based models with respect to robustness to affine transformations for classification on CIFAR10 and FashionMNIST. The methods we compare are CapsNet [35], EMCaps [17], LCaps [20], and SCN [11]. Similar to MNIST, we also created five different versions of train and test-set by randomly rotating data. Each model is trained on the five transformed versions of the training set separately, and then test each model on all five variations of the testing set, in the Table 1. In only seven out of 25 cases, SCN provide better accuracy (on CIFAR10), but its number of parameters are much higher than ours. From the results, we observe that to train and test the geometric transformations of input, WECapsule appears to a notably more robust choice. On the CIFAR10 experiments, SCN performs better than WECapsule on the untransformed data. However, WECapsule learns from train-time transformations better than SCN, and outperforming it in a large majority of the cases. We infer that the SCN contains a large number of parameters which allows capturing features that generalize better to transformations.

**Table 1.** Affine transformation experiments on CIFAR10 (left), and FashionMNIST (right)

| Training on untransformed data (0°) |              |              |              |              |              | Training on untransformed data (0°) |              |              |              |              |              |
|-------------------------------------|--------------|--------------|--------------|--------------|--------------|-------------------------------------|--------------|--------------|--------------|--------------|--------------|
| Method                              | 0            | 30°          | 45°          | 90°          | 180°         | Method                              | 0            | 30°          | 45°          | 90°          | 180°         |
| CapsNet                             | 67.41        | 57.57        | 45.34        | 37.69        | 34.23        | CapsNet                             | 91.57        | 62.43        | 48.78        | 36.29        | 31.70        |
| EMCaps                              | 62.23        | 50.76        | 43.18        | 32.92        | 33.76        | EMCaps                              | 90.24        | 64.67        | 49.53        | 35.42        | 32.26        |
| LCaps                               | 78.39        | 62.54        | 57.73        | <b>55.32</b> | 38.59        | LCaps                               | 86.56        | 68.05        | 45.79        | 43.83        | 41.59        |
| SCN                                 | 81.53        | 68.11        | <b>63.33</b> | <b>55.38</b> | 42.36        | SCN                                 | 93.39        | 72.21        | 58.37        | 49.64        | 47.93        |
| WECaps                              | <b>92.04</b> | <b>74.32</b> | <b>62.46</b> | <b>51.29</b> | <b>49.62</b> | WECaps                              | <b>95.27</b> | <b>74.52</b> | <b>67.33</b> | <b>61.38</b> | <b>52.11</b> |
| Training on transformed data (30°)  |              |              |              |              |              | Training on transformed data (30°)  |              |              |              |              |              |
| Method                              | 0            | 30°          | 45°          | 90°          | 180°         | Method                              | 0            | 30°          | 45°          | 90°          | 180°         |
| CapsNet                             | 71.29        | 68.57        | 62.42        | 56.45        | 47.81        | CapsNet                             | 92.63        | 86.32        | 69.54        | 57.86        | 45.17        |
| EMcaps                              | 68.53        | 62.74        | 59.38        | 55.14        | 47.23        | EMCaps                              | 92.08        | 85.57        | 68.39        | 55.40        | 42.35        |
| LCaps                               | 78.64        | 77.51        | 73.65        | 69.58        | 54.32        | LCaps                               | 84.29        | 81.03        | 75.23        | 70.84        | <b>66.35</b> |
| SCN                                 | 86.39        | 83.76        | 82.39        | <b>79.56</b> | 68.79        | SCN                                 | 92.34        | 92.48        | 87.54        | <b>73.82</b> | 57.86        |
| WECaps                              | <b>90.78</b> | <b>88.64</b> | <b>85.72</b> | <b>76.43</b> | <b>70.53</b> | WECaps                              | <b>94.72</b> | <b>93.38</b> | <b>89.75</b> | <b>72.31</b> | <b>65.72</b> |
| Training on transformed data (45°)  |              |              |              |              |              | Training on transformed data (45°)  |              |              |              |              |              |
| Method                              | 0            | 30°          | 45°          | 90°          | 180°         | Method                              | 0            | 30°          | 45°          | 90°          | 180°         |
| CapsNet                             | 72.36        | 68.56        | 66.94        | 59.41        | 48.93        | CapsNet                             | 87.94        | 86.25        | 86.19        | 81.70        | 54.39        |
| EMCaps                              | 69.42        | 65.29        | 63.45        | 55.76        | 47.32        | EMCaps                              | 86.32        | 85.32        | 84.74        | 79.52        | 53.76        |
| LCaps                               | 82.81        | 81.22        | 78.41        | 75.46        | 68.59        | LCaps                               | 88.27        | 86.94        | 81.56        | 73.62        | 59.25        |
| SCN                                 | 83.27        | <b>82.45</b> | 78.34        | <b>77.53</b> | 70.96        | SCN                                 | 93.44        | 93.16        | 92.73        | <b>88.36</b> | 63.84        |
| WECaps                              | <b>85.43</b> | <b>81.99</b> | <b>80.46</b> | <b>76.54</b> | <b>73.90</b> | WECaps                              | <b>94.69</b> | <b>94.38</b> | <b>94.41</b> | <b>87.67</b> | <b>65.51</b> |
| Training on transformed data (90°)  |              |              |              |              |              | Training on transformed data (90°)  |              |              |              |              |              |
| Method                              | 0            | 30°          | 45°          | 90°          | 180°         | Method                              | 0            | 30°          | 45°          | 90°          | 180°         |
| CapsNet                             | 68.24        | 62.51        | 62.27        | 59.54        | 53.76        | CapsNet                             | 86.71        | 85.29        | 85.12        | 84.97        | 59.14        |
| EMCaps                              | 67.32        | 60.80        | 59.72        | 57.66        | 51.41        | EMCaps                              | 85.49        | 84.93        | 84.25        | 83.64        | 58.92        |
| LCaps                               | 81.20        | 79.38        | 79.65        | 78.19        | 76.59        | LCaps                               | 79.51        | 79.35        | 79.61        | 78.36        | 75.86        |
| SCN                                 | <b>84.31</b> | 83.08        | <b>82.64</b> | 80.76        | 76.45        | SCN                                 | 93.49        | 93.37        | <b>92.86</b> | 91.23        | 71.30        |
| WECaps                              | <b>84.24</b> | <b>83.46</b> | <b>82.26</b> | <b>82.43</b> | <b>79.65</b> | WECaps                              | <b>94.26</b> | <b>94.13</b> | <b>92.58</b> | <b>92.72</b> | <b>91.58</b> |
| Training on transformed data (180°) |              |              |              |              |              | Training on transformed data (180°) |              |              |              |              |              |
| Method                              | 0            | 30°          | 45°          | 90°          | 180°         | Method                              | 0            | 30°          | 45°          | 90°          | 180°         |
| CapsNet                             | 63.29        | 61.66        | 62.73        | 59.28        | 58.90        | CapsNet                             | 89.26        | 86.90        | 85.48        | 85.39        | 84.77        |
| EMCaps                              | 61.53        | 57.32        | 58.36        | 58.49        | 57.76        | EMCaps                              | 85.98        | 85.36        | 85.71        | 84.33        | 84.29        |
| LCaps                               | 80.98        | 80.46        | 81.07        | 80.89        | 78.47        | LCaps                               | 81.27        | 80.93        | 79.24        | 79.53        | 78.52        |
| SCN                                 | 82.25        | 81.48        | 81.34        | 81.56        | 81.43        | SCN                                 | 91.60        | 92.07        | 91.35        | 91.51        | 91.66        |
| WECaps                              | <b>82.71</b> | <b>82.59</b> | <b>82.33</b> | <b>82.16</b> | <b>82.41</b> | WECaps                              | <b>94.52</b> | <b>94.12</b> | <b>93.56</b> | <b>93.78</b> | <b>93.61</b> |

## References

1. Benamou, J.D., Carlier, G., Cuturi, M., Nenna, L., Peyré, G.: Iterative bregman projections for regularized transportation problems. SIAM J. Scientific Computing **37**(2), A1111–A1138 (2015)
2. Cuturi, M.: Sinkhorn distances: Lightspeed computation of optimal transport. In: Proc. Adv. Neural Inf. Process. Syst. (NeurIPS). pp. 2292–2300 (2013)
3. Peyré, G., Cuturi, M., Solomon, J.: Gromov-wasserstein averaging of kernel and distance matrices. In: Proc. Int. Conf. Mach. Learn. (ICML). pp. 2664–2672 (2016)
